# Supplementary material for: Nonparametric estimation of highest density regions for COVID-19
Source: arXiv:2010.14340 source file (2020-11-20)
Supplement: Supplementary file 1 [file supplementary_material.pdf]

# Supplementary material: Nonparametric estimation of highest density regions for COVID-19

## 1 Interactive representation of daily evolution of COVID-19 confirmed cases distribution around the world

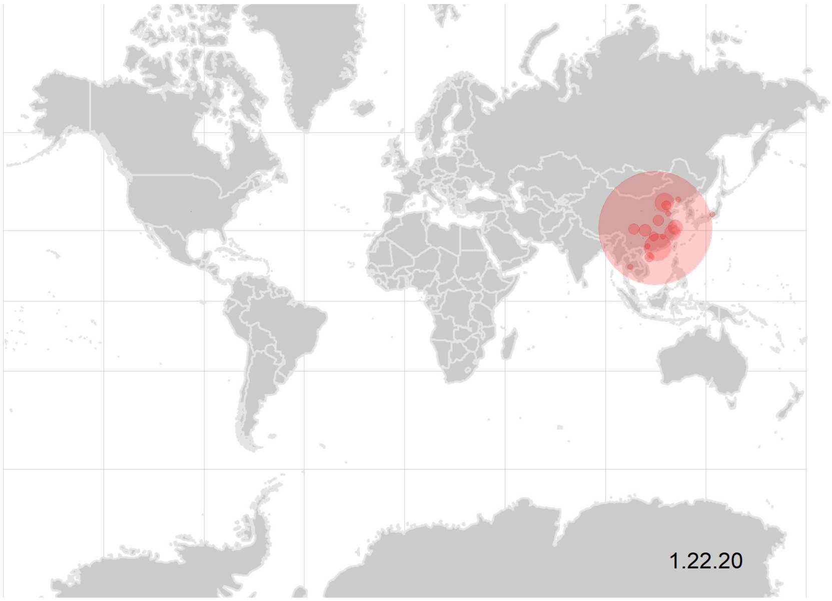


Play/Pause

Figure 1: Time evolution of COVID-19 cases distribution around the world from January to May 2020.

## 2 Interactive representation of HDRs for COVID-19

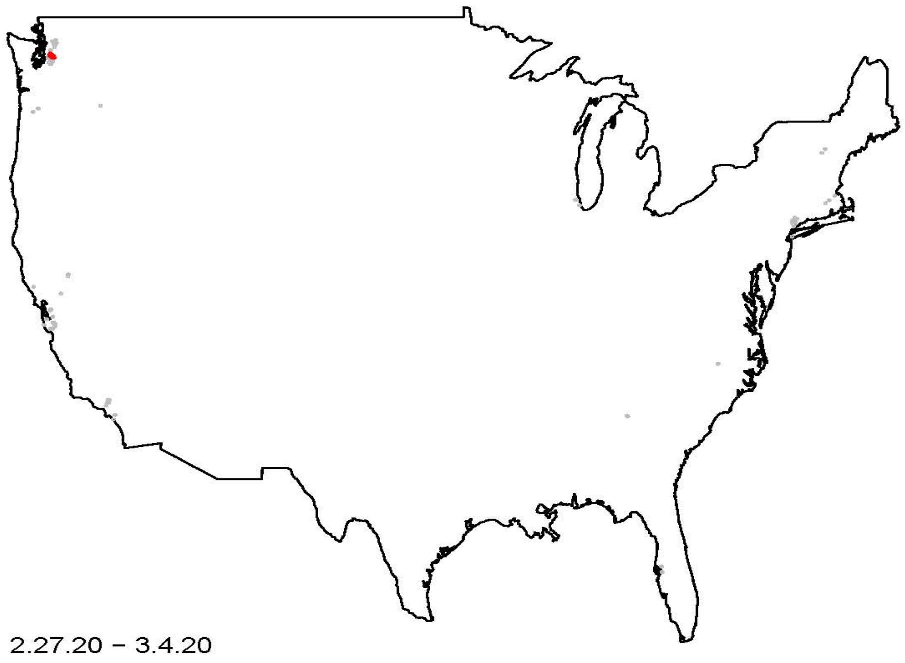


Play/Pause

Figure 2: Space-time evolution of HDRs when $\tau = 0.9$ for confirmed COVID-19 cases in United States by week from February to May 2020.

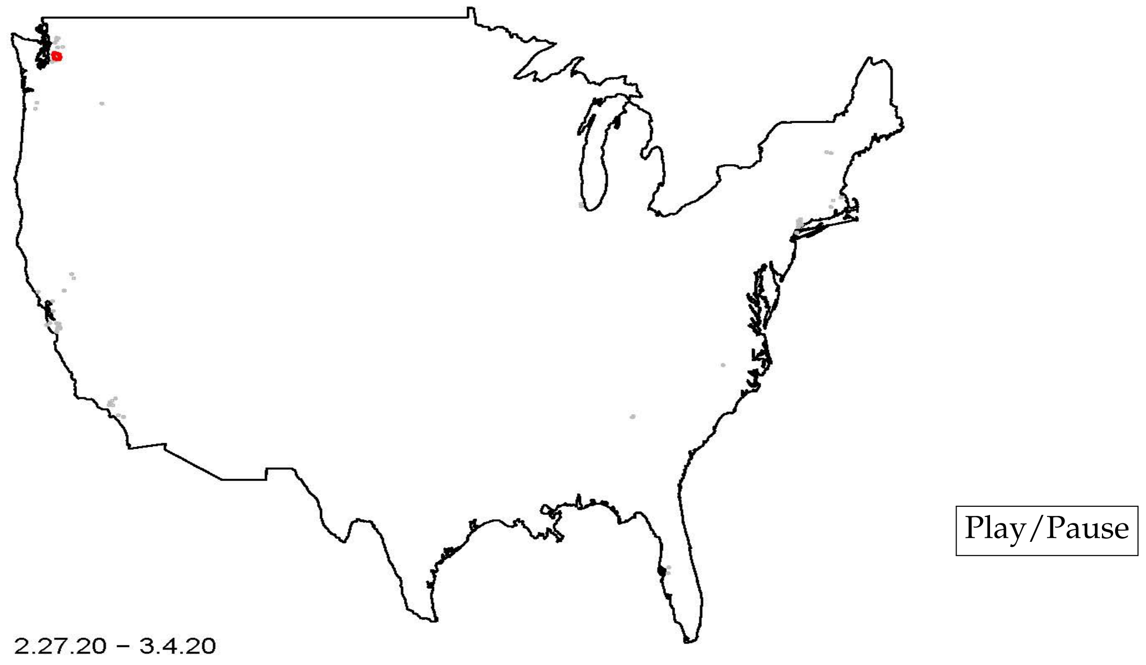


Figure 3: Space-time evolution of HDRs when $\tau = 0.8$ for confirmed COVID-19 cases in United States by week from February to May 2020.

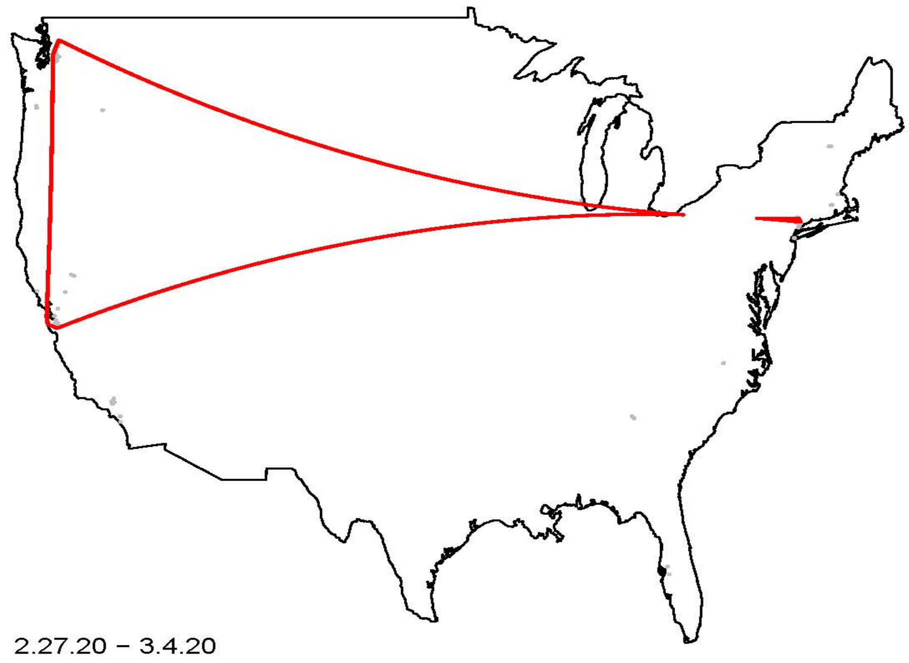


Play/Pause

Figure 4: Space-time evolution of HDRs when $\tau = 0.5$ for confirmed COVID-19 cases in United States by week from February to May 2020.
